# Supplementary material for: PERKS: a Locality-Optimized Execution Model for Iterative Memory-bound GPU Applications
Source: arXiv:2204.02064 source file (2023-05-12)
Supplement: Supplementary file 1 [file 08_appendix.tex]

%% Appendix
% \newpage
\appendix
\section{{Why PERKS is Feasible in the latest Nvidia GPUs}}\label{sec:whyperks}

This section summarizes the three hardware development in GPUs that make PERKS feasible now. First, a fewer amount of warps is required for CUDA runtime to hide the latency effectively, since the latency of most compute, data, and control operations dropped significantly in recent generations of GPUs~\cite{jia2018dissecting}. We discussed the sufficiency of low occupancy in Section~\ref{sec:perconcurrency}. 

%Also, we can find traces in literature. On one side, the CUDA programming guide~\cite{nvidia2019programming} shows a trend of reducing throughput per stream multiprocessor. On the other hand, if we compare the latency result in existing microbenchmarks~\cite{wong2010demystifying,jia2018dissecting} we can also observe a reduction in instruction latency. Both trends result in a lower hardware concurrency per stream multiprocessor in newer generation GPUs. 

Second, a new explicit device-wide synchronization API released in CUDA 9.0 (2017) provides the possibility to reuse on-chip resources between device-wide barriers with lower overhead (Section~\ref{sec:backsync}). The overhead is further reduced in the newer GPU generations~\cite{amperewhite}.

Third, as reported by Nvidia developer guides~\cite{nvidiaa100}, on-chip resources have increased from 17.5 MB in P100 (2016) to 44.29 MB in A100 (2020) ($2.53$x larger in 4 years). This further benefits PERKS since it increases the capacity for caching. 

% Zhang etc.~\cite{zhang2020study} did a comprehensive research on this and showed that the difference in overhead between explicit device-wide synchronization and implicit device-wide synchronization is largely negligible. 

\begin{table}[t]
    \centering
    \caption{The memory related parameters of the latest Nvidia GPUs\cite{nvidiaa100}}% SM is Steam Multiprocessor}
    \resizebox{\linewidth}{!}{
    \begin{tabular}{?l?c|c|c?}\tbhline
    \textbf{Feature}    & \textbf{P100} & \textbf{V100}  & \textbf{A100}  \\\hline
    \textbf{Shared memory}~\tablefootnote{\emph{Shared memory} is a configurable portion of L1 cache that can be used as a user-managed scratchpad memory} 
    & 3.5 MB & 7.5 MB & 17.29 MB \\
    \textbf{Register files} &14 MB &20MB&27MB\\
    \textbf{L2 cache }    & 4 MB & 6 MB  & 40 MB  \\
    \textbf{Memory bandwidth}    & 720 GB/s & 900 GB/s  & 1555 GB/s  \\\hline
    % \textbf{Time}    &   &  & \\
    % \textbf{(Fill $50\%$ of register files)}    &  10.19 ns & 11.65 ns & 9.10 ns \\\hline
    \end{tabular}
    \label{tab:gpu_loadsmltc}
    }
\end{table}
\section{PERKS and CUDA Considerations}
\subsection{Restrictions of Synchronization APIs}
PERKS highly relies on cooperative groups related APIs (supported since CUDA 9.0~\cite{nvidia2021api}). Currently, the API does not allow over-subscription, i.e., one needs to explicitly assign workload to blocks and threads to expose enough parallelism to the device. However, it is worth mentioning that this API does not limit the flexibility, as different kernels can still run concurrently in a single GPU, as long as they as a whole doesn't exceed the hardware limitation.

\subsection{New Features in Nvidia Ampere}
The Nvidia Ampere generation of GPUs introduced two new features that have the potential to improve the performance of PERKS. Namely, asynchronous copy for shared memory and L2 cache residency control~\cite{nvidiaa100}. When testing asynchronous copy to cache in PERKS, we did not observe noticeable performance difference. For L2 cache residency control, we experimented with setting the input and halo region to be persistent. We observed $8\%$ slowdown and no change in performance, respectively. Accordingly, we do not use those new features in our PERKS implementations.

\subsection{Register pressure in PERKS} 
One concern with PERKS is that kernels might run into register pressure if the compiler is not optimally reusing registers for different time steps, potentially affecting concurrency and penalizing performance. To illustrate this issue, take a high register-pressure 2D 25-point double precision Jacobi stencil as an example. The shared memory optimized baseline version (SM-OPT) uses $78$ registers per thread, yet the PERKS version uses $112$ registers\footnote{We gathered the number of registers used by finding the maximum number of registers available as cache before spilling with "\_\_launch\_bounds\_\_" instruction. Register spilled can be indicated by '-Xptxas "-v -dlcm=cg"' flag.}. Similar behavior is also observed in other stencil benchmarks. Reducing the occupancy while maintaining the concurrency --as mentioned in the previous section-- reduces the impact of this compiler's inefficiency in register reuse in all the benchmarks we report in the results section. In the above example, at worst, $48$ registers among the maximum available $178$ registers per thread could not be used for caching data; it neither harms concurrency nor triggers register spilling. 

\begin{table}[t]
    \centering
    \caption{Register information of single precision 2d5pt and double precision 2ds25pt}
    \begin{tabular}{|c|c|c|}
    \hline
        TYPE & 2d5pt(f)  & 2ds25pt(d)  \\\hline
        SM-OPT            & 32  & 78 \\
        PERKS(SM-OPT)                    & 32  & 112\\
        PERKS(SM-OPT) with $D_{cache}^{sm}$& 32  & 126\\\hline
    \end{tabular}
    \label{tab:registeranalysis}
\end{table}

\section{Caching}
\subsection{Caching Policy}\label{sec:cachepolicy}

A caching policy is required to determine which portion of the domain (or data) to cache. When the entire domain (or data) can fit in register files and shared memory used for caching, the entire algorithm can run from the cache (this is particularly useful in the cases of strong scaling where per node domain size becomes smaller as the number of nodes grows). When only a fraction of the domain can be cached, a policy is required to select the data to prioritize for caching. In the following sections, we elaborate on the caching policy.

\subsubsection{Considerations for dependency between threads Blocks} 
Algorithms that do not require dependency between the thread blocks can use the cache space most efficiently because all the load and store transactions to global memory can be eliminated. The dependencies within the thread block are resolved by using either the shared memory or shuffle operations.

In iterative solvers, there is often neighbor dependency (ex: a stencil kernel where a cell update relies on values computed in neighboring threads). In such a case, caching the results of the threads at the interior of the CUDA thread blocks eliminates the stores and loads from global memory. The threads at the boundary of threads blocks would, however, continue to store and load from global memory (since the shared memory scope is the thread block). When the capacity of cache is large enough, w.r.t. the domain size to be cached, the performance drawback would be negligible. 

\subsubsection{Identifying which data gets priority to be cached}

In many cases, the capacity of register files and shared memory is limited, i.e., it is impossible to cache the entire domain/input. In cases where all the domain/input array elements are accessed at the same frequency, one could assume it is unnecessary to use a cache policy that prioritizes specific parts of the domain/input. However, this is not always true.

Take iterative stencil as an example. The data managed by the threads at the boundary of the thread block is stored to main memory to be accessed by the neighboring threads blocks in the following iterations; caching those boundary elements saves one load operation. On the other hand, data at the interior of the thread block is not involved in inter thread block dependency; caching saves one load and one store operation. Finally, data in the halo region is updated at each time step; there is no benefit in caching the layers in the halo region. To conclude, the priority in caching yielding the highest reuse would be: {\footnotesize $Data_{no\_inter\_TB\_dependency}>Data_{inter\_TB\_dependency}$}, i.e., the priority is to cache the data of the interior threads of the thread block, followed by the data of the threads at the boundary of the thread block, and no caching for the halo region.

For other iterative solvers, such as conjugate gradient, there are different data arrays that could be potentially cached, unlike a single domain array in stencils. The cacheable variables and usage per array element for the conjugate gradient solver are as follows: a) one load and no stores for the matrix {$\mathbf{A}$}, and b) three loads and one store for the residual vector {$\mathbf{r}$}. So by assuming that each operation accesses data in a coalesced access pattern, it would be more effective to cache vector {$\mathbf{r}$}. As a result, the ideal cache priority is {\footnotesize$\mathbf{r}>\mathbf{A}$}.

To summarize, while PERKS does not touch on the compute part of the original kernel, attention should be given to identifying the ideal caching policy for each solver implemented as PERKS. That being said, one could assume this step can be automated by using a dedicated profile-guided utility (or even sampling from the profiler directly) to aid the user in swiftly identifying an ideal caching policy, based on the access patterns and frequency of access of data arrays in the solver.

\subsection{Detailed Results}
\subsubsection{Where to Cache: Shared Mem., Registers, or Both?}

\label{sec:caching:where}
The intuition is that using both shared memory and registers would always be better (more cache-able space). The results show that this is usually the case. There can, however, be exceptions. For instance, in our observations, we see that for higher order stencils, using shared memory and registers is often not the ideal choice (presumably due to arising register pressure).

\subsubsection{What to Cache?}
\label{sec:what:cache}
We highlight important observations when varying the data to cache in the conjugate gradient solver. First, the implicit cache policy ($IMP$) achieves a geometric mean of $3.63$x and $1.21$x over Ginkgo for dataset sizes both within and (surprisingly) when exceeding L2 cache, respectively. This means \textbf{PERKS can gain speedup before applying any explicit caching policy} by getting hits in the L2 cache. Second, the speedup difference between caching the vector ($VEC$) or not is usually insignificant for most situations. This is likely because the vectors are generally not large enough to consume all available cache resources. Third, as expected, the general tendency is that the more PERKS caches, the more speedup there is. So we generally get the highest speedup with caching the matrix ($MAT$) or caching both the vector and matrix ($MIX$). The exception is in the case of single precision when the dataset sizes exceed L2 cache: we still get speedup from $MAT$ and $MIX$, though not the highest speedup. 
\subsubsection{What Should the End-user Do?}
\label{sec:summary:cache}
In summary, the cache location analysis for stencil and the cache policy analysis for conjugate gradient (which is a fairly complex solver) shows that a simple greedy approach of targeting the largest data arrays in as many caching resources as possible gives mostly the best performance. While there can be outliers, the simple greedy policy is, in most cases, effective enough, and also simple for end-users (since they only need to identify the arrays generating the most traffic).

\begin{figure}[t]
\centering
\includegraphics[width=\linewidth]{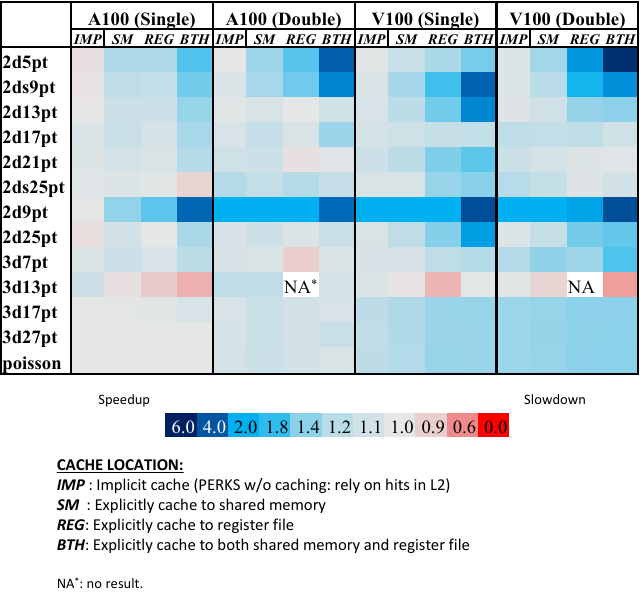}
\caption{Heatmap of speedup over non-PERKS baseline (SM-OPT) when caching data in different locations, for different stencils.}
\label{Fig:stheatmap}
\end{figure}

\begin{figure}[t]
\centering
\textcolor{white}
{
\frame
{\includegraphics[width=\linewidth]{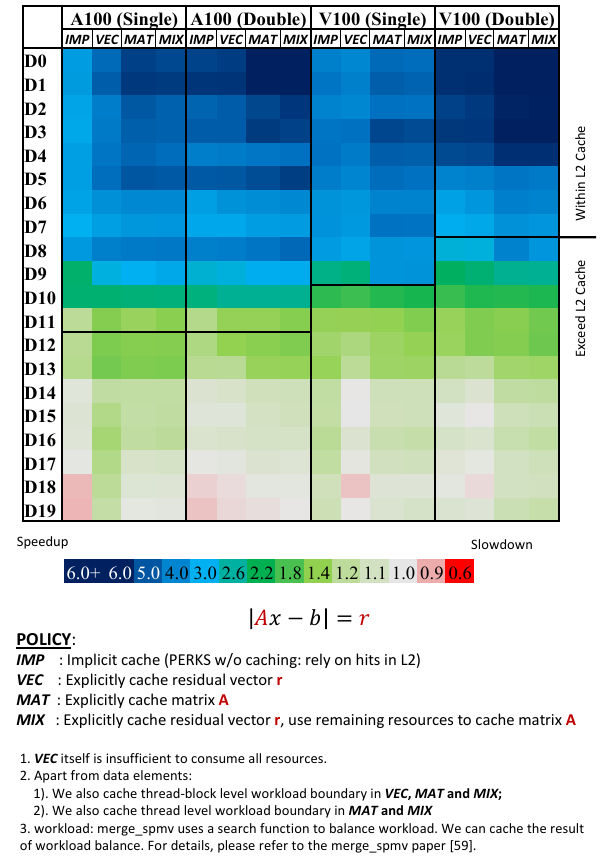}}}
\caption{ Heatmap of speedup over Ginkgo~\cite{anzt2020ginkgo} when using different caching policies in the conjugate gradient solver (iterative method to solve $Ax=b$).
}
\label{Fig:cgpolicy}
\end{figure}
\section{Performance Analysis}\label{appendix}

First, We propose a projection of achievable performance that we compare with measured results to detect abnormal behavior or implementation shortcomings. We relied on this projection to analyze our PERKS implementation quality (Section~\ref{sec:peakperform}).

Second, We identify the bounds on reducing concurrency before dropping performance and use concurrency to explain potential optimizations for further performance improvement (Section~\ref{sec:apdconan}). 

\textbf{We emphasize that:} we use the analysis to understand the quality of our implementation and address its implication on performance. However, the concurrency analysis is not a requirement for porting kernels to PERKS;  In contrast, end-users wishing to port the kernel to PERKS need only to satisfy the concurrency requirements by setting the device occupancy to minimum occupancy while maintaining performance (Section~\ref{sec:enduser}). 

Finally, we also provide an empirical performance model for end-users in the large domain, which projects the speedup before applying PERKS without the knowledge of concurrency analysis (Section~\ref{sec:empmodel}).

\subsection{Overview}
This performance analysis relies on three performance attributes: a) measured performance $\mathbb{M}$ of our PERKS implementation, b) the projected peak performance $\mathbb{P}$ achievable on a given GPU,  and c) the efficiency function $\mathfrak{E()}$ describing the efficiency of the given kernel running on the device.
More specifically, $\mathfrak{E()}$ is a function of the concurrency exposed by the software $\mathbb{C}_{sw}$ and the concurrency required by the hardware $\mathbb{C}_{hw}$. The relation of measured performance to projected peak performance becomes:
\begin{equation}\footnotesize
   \mathbb{M}  =  \mathbb{P}\times \mathfrak{E(} \mathbb{C}_{sw},\mathbb{C}_{hw}\mathfrak{)}
    \label{eqt:basic}
\end{equation}
We discuss projected peak performance in the following section. A detailed discussion of the efficiency and concurrency functions is in Section~\ref{sec:apdperconcurrency}.

\subsection{Projecting Peak Achievable Performance}\label{sec:peakperform}
Details can be referred to Section~\ref{sec:howperksreduces}.

\subsection{{Quality of the implementation}}

The roofline-like model we propose suffers from the same limitations of the roofline model, e.g., it has an implicit assumption of perfect overlap of compute and memory accesses. Additionally, inaccuracies can arise from the L2 concurrency issues we discussed in Section~\ref{sec:perconcurrency}. The projected peak performance is effective in serving the purposes of identifying unanticipated performance gaps and guiding our occupancy reduction. That being said, it is important to note that projected peak performance showed is taken as an indicator of the bound on performance improvement and not as accurate performance prediction. %In large-domain stencils, we observed $64\%$ ($36\%\sim85\%$) of the projected peak. In the small-domain stencils, we observe $59\%$ ($34\%\sim97\%$) of the projected peak. 

%The roofline-like model we proposed reveals the achievable performance. It can help us understand the implementation quality. 
In large-domain stencils, we achieved $64\%$ ($36\%\sim84\%$) of the projected peak. In the small-domain stencils, we achieved $59\%$ ($34\%\sim108\%$) of the projected peak. The $100+\%$ performance likely comes from L2 cache that we didn't include in the model.

\subsection{Concurrency and Micro-benchmarks}\label{sec:apdperconcurrency}
Reducing device occupancy increases the availability of resources to be used for caching in PERKS (as illustrated earlier in Figure~\ref{Fig:showcase}). On the contrary, reducing occupancy can lead to lower device utilization. To effectively implement PERKS, one has to reduce the occupancy as much as possible without scarifying performance. Inspired by the findings of Volkov~\cite{volkov2010better}, we assume that the efficiency function $\mathfrak{E}$ reaches its peak point when the code provides enough concurrency to saturate the device (irrespective of the occupancy):
\begin{equation}\footnotesize
    \mathfrak{E}(\mathbb{C}_{sw},\mathbb{C}_{hw})=100\%, \text{if } \forall \mathbb{C}_{sw}\geq \mathbb{C}_{hw}
    \label{eqt:efficiency}
\end{equation}

Where $\mathbb{C}_{sw}(\mathbb{OP})$ is the minimum number of concurrently executable instructions of the operation $\mathbb{OP}$ exposed by the launched kernel, and $\mathbb{C}_{hw}(\mathbb{OP})$ is the maximum numbers of instructions of the operation $\mathbb{OP}$ that the device is capable of handling concurrently. Because this paper mainly focuses on memory-bound applications, the $\mathbb{OP}$ referred to in this paper are limited to data access operations, i.e. global memory load/store $\mathbb{C}(\mathbb{GM})$, shared memory load/store $\mathbb{C}(\mathbb{SM})$, and L2 cache load/store $\mathbb{C}(\mathbb{L}2)$.

\subsubsection{Measuring $\mathbb{C}_{sw}^{SMX}$} $\mathbb{C}_{sw}^{SMX}(\mathbb{OP})$, the kernel concurrency at the streaming multi-processor (SMX) level, can be computed based on the concurrency exposed by the threads of a thread block $\mathbb{C}_{sw}^{TB}(\mathbb{OP})$ and number of concurrently running thread blocks per stream multiprocessor {\footnotesize$TB/SMX$}:  {\footnotesize$\mathbb{C}_{sw}^{SMX}(\mathbb{OP})=\mathbb{C}_{sw}^{TB}(\mathbb{OP})\cdot TB/SMX$}.

\subsubsection{Measuring $\mathbb{C}_{hw}$} According to Little's Law~\cite{Little1961APF}, the hardware concurrency $\mathbb{C}_{hw}$ can be determined by the throughput $\mathbb{THR}$ and latency $\mathbb{L}$\cite{volkov2010better}: 
\begin{equation}\footnotesize
    \mathbb{C}_{hw}(\mathbb{OP})=\mathbb{THR(OP)} \cdot \mathbb{L(OP)}
\end{equation}

The throughput $\mathbb{THR}$ for different data access operations are available in Nvidia online documents~\cite{nvidia2019programming,amperewhite}. We measure the latency $\mathbb{L}$ with commonly used microbenchmarks~\cite{wong2010demystifying,mei2014benchmarking,zhang2017understanding}. Table~\ref{tab:concurrency} shows the detailed results in V100 and P100. We can further induce the minimal concurrency necessary for accessing global memory. The detailed results are displayed in Table~\ref{tab:lowoccupancy}.

\begin{comment}
	Latency of shared memory and L2 Cache can be tested with microbenchmark provided by previous research~\cite{wong2010demystifying,mei2014benchmarking}. But these works\cite{wong2010demystifying,mei2014benchmarking} test global memory latency with a metrics of cycle, which do not reflect its latency in second due to dynamic frequency. We thereby combine Mei etc.'s~\cite{mei2014benchmarking} microbenchmark Zhang etc's research~\cite{zhang2017understanding} to test $L_{global}$ with CPU clock. The alternative measurement is to manually set frequency to be static and use the existing microbenchmark and latency in cycle and deduce its latency in second from the frequency. However, we found that the latency varies as the frequency varies; the latency of some operation involved in global memory access can be affected by the GPU uncore frequency. The CPU measured global memory latency with default dynamic frequency setting is reported in this paper. $Thr$, $L$ and $C$ of memory in A100 and V100 is gathered in Table~\ref{tab:concurrencysm}, Table~\ref{tab:concurrencyl2} and Table ~\ref{tab:concurrencygm}. 
\end{comment}

% \begin{comment}
\begin{table}[t]
	\caption{Throughput and latency of relevant operations on A100 and V100 GPUs}
    \centering
	\begin{tabular}{|c|c|c|}
	\hline
	 & A100&V100\\\hline
	\multicolumn{3}{|c|}{ Shared memory}\\\hline
	$\mathbb{THR}(\mathbb{SM})(B/cycle) $&128&128\\
	$\mathbb{L}(\mathbb{SM})(cycle)$ &28&26\\
	$\mathbb{C}^{SMX}_{hw}(\mathbb{SM}) (B)$ &3584&3328\\\hline
	\multicolumn{3}{|c|}{Global memory}\\\hline
	$\mathbb{THR}(\mathbb{GM})(GB/s) $ & 1555   & 900\\
	$\mathbb{L}(\mathbb{GM})(ns)$      & 403.28 & 286.17\\
	 $\mathbb{C}_{hw}(\mathbb{GM})(B)$& 627101 & 257553\\
	$\mathbb{C}^{SMX}_{hw}(\mathbb{GM})(B)$  & 5807   & 3220\\\hline	
	
	\multicolumn{3}{|c|}{L2 Cache}\\\hline
	$\mathbb{THR}(\mathbb{L}2)(B/cycle) $ & 5120   & 2048\\
	$\mathbb{L}(\mathbb{L}2)(cycle)$      & 218/384 & 200\\
	$\mathbb{C}_{hw}(\mathbb{L}2)(B)$& 1541120 & 409600\\
	$\mathbb{C}^{SMX}_{hw}(\mathbb{L}2)(B)$ & 14270   & 5120\\\hline	
	\end{tabular}
	\label{tab:concurrency}
\end{table} 
% 
\begin{comment}
\begin{table}[t]
	\caption{Hardware concurrency of memory access for double precision values per stream multiprocessors (SMX) on P100, V100, and A100 GPUs}
% \scriptsize
    \centering
	\begin{tabular}{|c|c|c|}
	\hline
	&\textbf{V100}&\textbf{A100}\\\hline
% 	\multicolumn{4}{|c|}{\textbf{Global memory}}\\\hline
	\textbf{$\mathbb{THR}$/SMX(GB/s)}~\cite{amperewhite}        & 12       & 15 \\
	\textbf{$\mathbb{L}$ (ns)}                & 286       & 403 \\
	\textbf{$\mathbb{C}_{hw}$/SMX (B)}      & 3220      & 5807   \\
    % $\mathbb{C}^{SMX}_{hw}(Double)$ & 624   & 432       & 764   \\
  \textbf{ Min Occupancy($ILP=1$)}  \tablefootnote{Min Occupancy is deduced by assuming that only using TLP for parallelism, and assuming that thread block size is 128}                   & 25\%  & 37.5\%     \\\hline	
	\end{tabular}
	\label{tab:lowoccupancy}
% 	{\footnotesize * Min Occupancy is deduced by assuming that only using TLP for parallelism}
\end{table} 
\end{comment}
% 
\begin{table}[t]
	\caption{Hardware concurrency of memory access for double precision values per stream multiprocessors (SMX) on P100, V100, and A100 GPUs}
% \scriptsize
    \centering
	\begin{tabular}{|c|c|c|c|}
	\hline
	 & \textbf{P100}&\textbf{V100}&\textbf{A100}\\\hline
% 	\multicolumn{4}{|c|}{\textbf{Global memory}}\\\hline
	\textbf{$\mathbb{THR}$/SMX(GB/s)}~\cite{amperewhite}       & 13    & 12       & 15 \\
	\textbf{$\mathbb{L}$ (ns)}                & 384   & 286       & 403 \\
	\textbf{$\mathbb{C}_{hw}$/SMX (B)}      & 4992  & 3220      & 5807   \\
    % $\mathbb{C}^{SMX}_{hw}(Double)$ & 624   & 432       & 764   \\
  \textbf{ Min Occupancy($ILP=1$)}  \tablefootnote{Min Occupancy is deduced by assuming that only using TLP for parallelism, and assuming that thread block size is 128}                 & 31.25\%  & 25\%  & 37.5\%     \\\hline	
	\end{tabular}
	\label{tab:lowoccupancy}
% 	{\footnotesize * Min Occupancy is deduced by assuming that only using TLP for parallelism}
\end{table}

\subsection{Concurrency Analysis}
\label{sec:apdconan}

In this section, we briefly describe how we analyze the concurrency to reduce the occupancy of the original kernel in order to release resources for caching while sustaining performance. We conduct a static analysis to extract the data movement operations in the kernel. Note that we account for any barriers in the original kernels that could impact the concurrency of operations, i.e., we do not combine operators/instructions from before and after the barrier when we count the operators. Finally, we apply efficient function $\mathfrak{E()}$ (Equation~\ref{eqt:efficiency}) to identify the least occupancy we could drop to before the concurrency starts to drop. 

For example, we did a static analysis of a single precision 2D 5-point Jacobi stencil kernel to conduct a concurrency analysis. It is worth mentioning that the baseline kernel we use is fairly complex since it is highly optimized by using shared memory to reduce traffic to global memory to its minimum~\cite{maruyama2014optimizing}. The results are summarized in Table~\ref{tab:concurrencyanalysis}. It shows that for this kernel, we could reduce the original occupancy to ${1/4}^{th}$ while maintaining performance.

To understand the gap between the projected upper-bound on achievable performance and the measured performance ($94.75/138.29=68.52\%$), we inspect the efficiency function $\mathfrak{E()}$. The results revealed that the concurrency for accesses in L2 cache, not global memory, is impacted by reducing occupancy on A100 in specific to the level that affects performance notably. More particularly, access to global memory for the halo region garners a high L2 cache hit rate. This effectively means that higher concurrency is necessary to saturate the L2 cache when hit rates are high. To confirm, we manually doubled the concurrency $\mathbb{C}^{TB}_{sw}$: the performance increased to 123.94 GCells/s with TB/SMX=1 (from $68.52\%$ up to $89.6\%$).

\begin{table}[t]
    \centering
    \caption{Concurrency analysis of global memory accesses of a single precision 2D-5point Jacobi stencil kernel running on A100 (1000 time-steps on $3072^2$ domain)}
    \resizebox{\linewidth}{!}{
        \begin{tabular}{?c?c|c|c|c|c?}
        \tbhline
            \multirow{2}{*}{$\tfrac{TB}{SMX}$}  & Used Reg. & Unused Reg. & GM Load & GM Store & Measured\\
              & /SMX  &/SMX    & op/SMX & op/SMX  & GCells/s\\\tbhline
            \textit{1} & 32KB  & 224KB  & 2580 & 2048 & 94.75\\
            \textit{2} & 64KB   & 192KB & 5160 & 4096 & 133.24\\
            \textit{8} & 256KB  & 0KB   & 20640 & 16384 & 138.29\\\tbhline
        \end{tabular}
    }
    \label{tab:concurrencyanalysis}
\end{table}

\subsection{Empirical Performance Model}\label{sec:empmodel}

Based on the performance analysis, we further deduce an empirical performance model for end-user. This model can help decide whether to apply PERKS without the knowledge of performance analysis. 

\textbf{Assumption:} PERKS does not change the efficiency of any implementations. If parallel parameters are equal to each other, $\mathfrak{E}_{PERKS}=\mathfrak{E}_{ori}$. According to Equation~\ref{eqt:basic}, we can deduce that:

\begin{equation}\footnotesize
    \mathbb{M}_{PERKS}=\mathbb{M}_{ori} \times \frac{\mathbb{P}_{PERKS}}{\mathbb{P}_{ori}}
    \label{eqt:projection}
\end{equation}

Additionally, in large domain/input size, assuming that the overhead of handling dependency is negligible, we can get:

\begin{equation}\footnotesize
\begin{aligned}
    \mathbb{M}_{PERKS}&=\mathbb{M}_{ori} \times \frac{1}{1-Per_{cache}}
\end{aligned}
\label{eqt:projectionLarge}
\end{equation}

For example, in 2D 5-point Jacobian stencil implementation, we set thread block=256. In baseline (SM-OPT), the default thread block per stream multiprocessor ($TB/SM$) is 8. Yet, after transforming the code to PERKS, the max $TB/SM$ is 2. We measured different $TB/SM$ settings for baseline and PERKS and put them in Table~\ref{tab:projection}. We also use Equation~\ref{eqt:projectionLarge} to project the performance based on the percentage of region cached and put the result in the same Table. 

\begin{table}[t]
    \centering\small
    \caption{Single precision $3702\times3702$ 2D 5-point Jacobian stencil in A100, performance of SM-OPT, PERKS and the performance projection}
    \begin{tabular}{|c|c|c|c|c|c|}
    \hline
        \multirow{2}{*}{$\tfrac{TB}{SM}$}  & SM-OPT & $Per_{cache}$ & Projection & PERKS&Accuracy\\
          & GCells/s && GCells/s & GCells/s&\\\hline
        1 & 94.87   & 77.34\%
        & 418.73& 357.79& 85.44\%\\
        2 & 133.41  & 79.69\% & 656.78& 444.55& 67.69\%\\ 
        8 & 137.65  & -       & - & -&-\\\hline
    \end{tabular}
    \label{tab:projection}
\end{table}

According to Table~\ref{tab:projection}, the Projection Model's accuracy is generally more than 67\%. So, this model can anticipate the potential speedup of applying PERKS without the knowledge of concurrency~\cite{volkov2010better}.

\section{Source code of PERKS-based 3d7pt stencil}
The PERKS-based 3d 7-pt stencil kernel is presented in this section.

\begin{lstlisting}[language=C,rulecolor=\color{black}, basicstyle=\tiny, caption=PERKS-based 3D 7-pt stencil with switch of source/ destination from/ to global memory/ shared memory/ register,captionpos=t]
template<class REAL, int halo, int LOCAL_ITEM_PER_THREAD, int BLOCKDIM, int LOCAL_TILE_X,int SM_SIZE_Z, int REG_SIZE_Z,
          int REG_CACHESIZE_Z=1,          
          bool loadfrmcache=false, bool storetocache=false,
          bool isloadfrmreg=false, bool isstoretoreg=false,
          int REGY_SIZE=REG_Y_SIZE_MOD, int REGX_SIZE=2*halo+1>
__device__ void __forceinline__ process_one_layer (REAL * __restrict__ input, REAL * __restrict__ output, 
        REAL* smbuffer_buffer_ptr[SM_SIZE_Z],REAL r_smbuffer[REG_SIZE_Z][LOCAL_ITEM_PER_THREAD],int global_z, int p_y, int p_x,int width_z, int width_y, int width_x,int ps_y, int ps_x, int sm_width_x,int cpbase_y, int cpend_y, int index_y,int tid_x, int tid_y,stencilParaList,REAL* sm_space=NULL, int frmcachesmid_z=0, int tocachesmid_z=0,REAL  r_space[REG_CACHESIZE_Z][LOCAL_ITEM_PER_THREAD]=NULL, int frmcacheregid_z=0, int tocacheregid_z=0,REAL* boundary_buffer=NULL, int boundary_buffer_index_z=0, const int boundary_east_step=0, const int boundary_west_step=0,const int boundary_north_step=0, const int boundary_south_step=0,const int boundary_step_yz=0)
{
  #define LOCAL_TILE_Y (LOCAL_ITEM_PER_THREAD*BLOCKDIM/LOCAL_TILE_X)
  #define gdim_y (BLOCKDIM/LOCAL_TILE_X)

  if(!loadfrmcache)
  {
    global2sm<REAL, halo, halo, 1, halo+1+isBOX, halo+isBOX, LOCAL_ITEM_PER_THREAD, gdim_y, false, true>(input, smbuffer_buffer_ptr,   p_x, p_y, global_z, width_x, width_y, width_z,  sm_width_x, ps_x, ps_y, LOCAL_TILE_X,tid_x,tid_y);
  }
  else
  {
    _Pragma("unroll")
    for(int l_y=0; l_y<LOCAL_ITEM_PER_THREAD; l_y++)
    {
      int local_y=l_y+LOCAL_ITEM_PER_THREAD*tid_y;

      if(!isloadfrmreg)
      {
        smbuffer_buffer_ptr[halo+isBOX][(local_y+ps_y)*sm_width_x+ps_x+tid_x] = sm_space[frmcachesmid_z*LOCAL_TILE_X*LOCAL_TILE_Y+(local_y-0)*LOCAL_TILE_X+tid_x];
      }
      else
      {
        smbuffer_buffer_ptr[halo+isBOX][(local_y+ps_y)*sm_width_x+ps_x+tid_x] = r_space[frmcacheregid_z][l_y];
      }
    }
    // middle frm sm or reg. halo need special care
    for(int l_y=tid_x-isBOX; l_y<LOCAL_TILE_Y+isBOX; l_y+=LOCAL_TILE_X)
    {
      #pragma unroll
      for(int l_x=tid_y; l_x<halo; l_x+=LOCAL_TILE_Y/LOCAL_ITEM_PER_THREAD)
      {
        //east
        smbuffer_buffer_ptr[halo+isBOX][(l_y+0+ps_y)*sm_width_x+ps_x+l_x+LOCAL_TILE_X] = boundary_buffer[boundary_east_step + (boundary_buffer_index_z) * (LOCAL_TILE_Y+2*isBOX)*halo  + (l_y+isBOX) + l_x * (LOCAL_TILE_Y+2*isBOX)];
        //west
        smbuffer_buffer_ptr[halo+isBOX][(l_y+0+ps_y)*sm_width_x+ps_x-halo+l_x]  = boundary_buffer[boundary_west_step + (boundary_buffer_index_z) * (LOCAL_TILE_Y+2*isBOX)*halo  + (l_y+isBOX) + l_x * (LOCAL_TILE_Y+2*isBOX)];
      }
    }
    //north south
    {
      int l_x=tid_x;
      #pragma unroll
      for(int l_y=tid_y; l_y<halo; l_y+=BLOCKDIM/LOCAL_TILE_X)
      {
        //north
        smbuffer_buffer_ptr[halo+isBOX][(l_y+LOCAL_TILE_Y+ps_y)*sm_width_x+ps_x+l_x] = boundary_buffer[boundary_north_step + (boundary_buffer_index_z) * (LOCAL_TILE_X)*halo  + (l_x) + l_y * (LOCAL_TILE_X)];
        
        //south
        smbuffer_buffer_ptr[halo+isBOX][(l_y-halo+ps_y)*sm_width_x+ps_x+l_x]  = boundary_buffer[boundary_south_step + (boundary_buffer_index_z) * (LOCAL_TILE_X)*halo  + (l_x) + l_y * (LOCAL_TILE_X)];
      }
    }
    __syncthreads();
  }

  //sm2reg
  sm2regs<REAL, LOCAL_ITEM_PER_THREAD, 1+2*halo, 1+halo, halo, 0, halo*2,  LOCAL_ITEM_PER_THREAD, 1>(smbuffer_buffer_ptr, r_smbuffer, ps_y+index_y, ps_x,  sm_width_x, tid_x);

  REAL sum[LOCAL_ITEM_PER_THREAD];
  _Pragma("unroll")
  for(int l_y=0; l_y<LOCAL_ITEM_PER_THREAD; l_y++)
  {
    sum[l_y]=0;
  }
  //main computation
  computation<REAL,LOCAL_ITEM_PER_THREAD,halo,REG_Y_SIZE_MOD>( sum,  smbuffer_buffer_ptr, ps_y+index_y,  sm_width_x, tid_x+ps_x,  r_smbuffer, stencilParaInput);

  __syncthreads();
  if(!storetocache)
  {
    reg2global3d<REAL, LOCAL_ITEM_PER_THREAD>(sum, output, global_z, width_z,p_y+index_y, width_y, p_x, width_x,  tid_x);
  }  
  else
  { 
    if(!isstoretoreg)
    {
      int z_ind=(tocachesmid_z)*LOCAL_TILE_X*LOCAL_TILE_Y;
      _Pragma("unroll")
      for(int l_y=0; l_y<LOCAL_ITEM_PER_THREAD; l_y++)
      {
        int local_y=l_y+index_y;
        sm_space[z_ind+(local_y-0)*LOCAL_TILE_X+tid_x]  = sum[l_y];
      }
    }
    else
    {
      _Pragma("unroll")
      for(int l_y=0; l_y<LOCAL_ITEM_PER_THREAD; l_y++)
      {
        r_space[tocacheregid_z][l_y]=sum[l_y];
      }
    }
  }
  REAL* tmp = smbuffer_buffer_ptr[0];
  // smswap 
  _Pragma("unroll")
  for(int hl=1; hl<halo+1+isBOX; hl++)
  {
    smbuffer_buffer_ptr[hl-1]=smbuffer_buffer_ptr[hl];
  }
  smbuffer_buffer_ptr[halo+isBOX]=tmp;
  regsself3d<REAL,REG_SIZE_Z,LOCAL_ITEM_PER_THREAD>(r_smbuffer);

  #undef LOCAL_TILE_Y
  #undef gdim_y
}
\end{lstlisting}
\begin{lstlisting}[language=C,rulecolor=\color{black}, basicstyle=\tiny, caption=3D 7-pt stencil computation function,captionpos=t]
#define stencilParaT const REAL center=-1.67f;const REAL west[1]={0.162f};const REAL east[1]={0.161f}; const REAL north[1]={0.163f}; const REAL south[1]={0.164f}; const REAL bottom[1]={0.166f}; const REAL top[1]={0.165f};
template<class REAL, int RESULT_SIZE, int halo, int REGY_SIZE,  int REGZ_SIZE=2*halo+1, int REGX_SIZE=2*halo+1, int REG_BASE=halo, int SMZ_SIZE=halo+1+halo>
#define isBOX (0)
#define stencilParaList const REAL west[HALO],const REAL east[HALO],const REAL north[HALO],const REAL south[HALO],const REAL top[HALO], const REAL bottom[HALO], const REAL center
#define stencilParaInput  west,east,north,south,top,bottom,center
#define REG_Y_SIZE_MOD (LOCAL_ITEM_PER_THREAD)
__device__ void __forceinline__ computation(REAL result[RESULT_SIZE],REAL* sm_ptr[SMZ_SIZE], int sm_y_base, int sm_width, int sm_x_ind,REAL reg_ptr[REGZ_SIZE][RESULT_SIZE], stencilParaList)
{
    _Pragma("unroll")
    for(int l_y=0; l_y<RESULT_SIZE; l_y++)
    {
      _Pragma("unroll")
      for(int hl=0; hl<halo; hl++)
      {
        result[l_y]+=west[hl]*
              sm_ptr[0][sm_width*(l_y+sm_y_base) + sm_x_ind-1-hl];
        result[l_y]+=east[hl]*
          sm_ptr[0][sm_width*(l_y+sm_y_base) + sm_x_ind+1+hl];
        result[l_y]+=north[hl]*
          sm_ptr[0][sm_width*(l_y+sm_y_base+1+hl) + sm_x_ind];
        result[l_y]+=south[hl]*
          sm_ptr[0][sm_width*(l_y+sm_y_base-1-hl) + sm_x_ind];
        result[l_y]+=bottom[hl]*reg_ptr[REG_BASE-1-hl][l_y];
        result[l_y]+=top[hl]*reg_ptr[REG_BASE+1+hl][l_y];
      }
    }
    _Pragma("unroll")
    for(int l_y=0; l_y<RESULT_SIZE; l_y++)
    {
        result[l_y]+=center*reg_ptr[REG_BASE][l_y];
    }
}
\end{lstlisting}

\begin{lstlisting}[language=C,rulecolor=\color{black}, basicstyle=\tiny, caption=supplimentary function,captionpos=t]
template<class REAL, int halo, bool isInit=false, bool sync=true>
__device__ void __forceinline__ global2sm(REAL* src, REAL* sm_buffer, 
                                              int size, 
                                              int global_y_base, int global_y_size,
                                              int global_x_base, int global_x_size,
                                              int sm_y_base, int sm_x_base, int sm_width,
                                              int tid)
{
  //fill shared memory buffer
  _Pragma("unroll")
  for(int l_y=0; l_y<size; l_y++)
  {
    int l_global_y;
    if(isInit)
    {
      l_global_y=(MAX(global_y_base+l_y,0));
    }
    else
    {
      l_global_y=(MIN(global_y_base+l_y,global_y_size-1));
      l_global_y=(MAX(l_global_y,0));
    }
    #define  dst_ind (l_y+sm_y_base)*sm_width
      sm_buffer[dst_ind-halo+tid+sm_x_base]=src[l_global_y * global_x_size + MAX(global_x_base-halo+tid,0)];
      if(halo>0)
      {
        if(tid<halo*2)
        {  
          sm_buffer[dst_ind-halo+tid+blockDim.x+sm_x_base]=src[(l_global_y) * global_x_size + MIN(-halo+tid+blockDim.x+global_x_base, global_x_size-1)];
        }
      }

  }
  if(sync==true)
  {  
    __syncthreads();
  }
  #undef dst_ind
}
template<class REAL, int halo, int BASE_Z, int SIZE_Z, int SMSIZE, int SM_BASE_Z=BASE_Z,  int LOCAL_ITEM_PER_THREAD, int gdim_y, bool isInit=false, bool sync=true>
__device__ void __forceinline__ global2sm(REAL *src, REAL* smbuffer_buffer_ptr[SMSIZE],
                                          int gbase_x, int gbase_y, int gbase_z,
                                          int width_x, int width_y, int width_z,
                                          int sm_width_x, int sm_base_x,
                                          int sm_base_y,
                                          int tile_x, int tid_x, int tid_y)
{
  _Pragma("unroll")
  for(int l_z=0; l_z<SIZE_Z; l_z++)
  {
    int l_global_z;
    if(!isInit)
    {
        l_global_z = (MIN(gbase_z+l_z+BASE_Z,width_z-1));
    }
    else
    {
       l_global_z = (MAX(gbase_z+l_z+BASE_Z,0));
    }
    #pragma unroll
    for(int i=0; i<LOCAL_ITEM_PER_THREAD; i++)
    {
      int l_y=i+tid_y*LOCAL_ITEM_PER_THREAD-halo;
      int l_global_y = (MIN(gbase_y+l_y,width_y-1));
        l_global_y = (MAX(l_global_y,0));
        smbuffer_buffer_ptr[l_z+SM_BASE_Z][sm_width_x*(l_y+sm_base_y) + (tid_x-halo) + sm_base_x]=
            src[l_global_z*width_x*width_y+l_global_y*width_x+
            MAX((gbase_x+tid_x-halo),0)];
      if(tid_x<halo*2)
      {
          smbuffer_buffer_ptr[l_z+SM_BASE_Z][sm_width_x*(l_y+sm_base_y) + tid_x + tile_x-halo+sm_base_x]=
              src[l_global_z*width_x*width_y+l_global_y*width_x+
                MIN(gbase_x+tid_x-halo+tile_x,width_x-1)];
      }
    }
    if(gdim_y>=2*halo)
    {
      {
        if(tid_y<2*halo)
        {
          int l_y=tid_y+gdim_y*LOCAL_ITEM_PER_THREAD-halo;
          int l_global_y = (MIN(gbase_y+l_y,width_y-1));
            l_global_y = (MAX(l_global_y,0));
            smbuffer_buffer_ptr[l_z+SM_BASE_Z][sm_width_x*(l_y+sm_base_y) + (tid_x-halo) + sm_base_x]=
                src[l_global_z*width_x*width_y+l_global_y*width_x+
                MAX((gbase_x+tid_x-halo),0)];
          if(tid_x<halo*2)
          {
              smbuffer_buffer_ptr[l_z+SM_BASE_Z][sm_width_x*(l_y+sm_base_y) + tid_x + tile_x-halo+sm_base_x]=
                  src[l_global_z*width_x*width_y+l_global_y*width_x+
                    MIN(gbase_x+tid_x-halo+tile_x,width_x-1)];
          }
        }
      }
    }
    else if(gdim_y>=2)
    {
      if(tid_y<2)
      {
        #pragma unroll
        for(int i=0; i<halo; i++)
        {
          int l_y=i+2*tid_y+gdim_y*LOCAL_ITEM_PER_THREAD-halo;
          int l_global_y = (MIN(gbase_y+l_y,width_y-1));
            l_global_y = (MAX(l_global_y,0));
            smbuffer_buffer_ptr[l_z+SM_BASE_Z][sm_width_x*(l_y+sm_base_y) + (tid_x-halo) + sm_base_x]=
                src[l_global_z*width_x*width_y+l_global_y*width_x+
                MAX((gbase_x+tid_x-halo),0)];
          if(tid_x<halo*2)
          {
              smbuffer_buffer_ptr[l_z+SM_BASE_Z][sm_width_x*(l_y+sm_base_y) + tid_x + tile_x-halo+sm_base_x]=
                  src[l_global_z*width_x*width_y+l_global_y*width_x+
                    MIN(gbase_x+tid_x-halo+tile_x,width_x-1)];
          }
        }
      }
    }
    else
    {
      if(tid_y==0)
      {
        #pragma unroll
        for(int i=0; i<2*halo; i++)
        {
          int l_y=i+gdim_y*LOCAL_ITEM_PER_THREAD-halo;
          int l_global_y = (MIN(gbase_y+l_y,width_y-1));
            l_global_y = (MAX(l_global_y,0));
            smbuffer_buffer_ptr[l_z+SM_BASE_Z][sm_width_x*(l_y+sm_base_y) + (tid_x-halo) + sm_base_x]=
                src[l_global_z*width_x*width_y+l_global_y*width_x+
                MAX((gbase_x+tid_x-halo),0)];
          if(tid_x<halo*2)
          {
              smbuffer_buffer_ptr[l_z+SM_BASE_Z][sm_width_x*(l_y+sm_base_y) + tid_x + tile_x-halo+sm_base_x]=
                  src[l_global_z*width_x*width_y+l_global_y*width_x+
                    MIN(gbase_x+tid_x-halo+tile_x,width_x-1)];
          }
        }
      }
    }
  }
  if(sync)
  {
    __syncthreads();
  }
}

template<class REAL,int REG_SIZE_Z, int REG_SIZE_Y, 
                        int BASE_Z=0,  int BASE_Y=0, 
                        int SIZE_Z=REG_SIZE_Z, int SIZE_Y=REG_SIZE_Y>
__device__ void __forceinline__ global2regs3d(
  REAL*src, REAL reg_array[REG_SIZE_Z][REG_SIZE_Y],
  int global_z, int width_z,
  int global_y, int width_y,
  int global_x, int width_x,
  int tid_x)
{
  _Pragma("unroll")
  for(int l_y=0; l_y<SIZE_Y; l_y++)
  {
    int l_global_y = (MIN(global_y+l_y+BASE_Y,width_y-1));
    l_global_y = (MAX(l_global_y,0));
    _Pragma("unroll")
    for(int l_z=0; l_z<SIZE_Z ; l_z++)
    {
      int l_global_z = (MIN(global_z+l_z+BASE_Z,width_z-1));
        l_global_z = (MAX(l_global_z,0));
      reg_array[l_z+BASE_Z][l_y+BASE_Y] = src[l_global_z*width_x*width_y+l_global_y*width_x+
            ((global_x+tid_x))];
    }
  }
}
template<class REAL, int SIZE_Z, int SIZE_Y>
__device__ void __forceinline__ regsself3d(
  REAL reg_array[SIZE_Z][SIZE_Y])
{
  _Pragma("unroll")
  for(int l_y=0; l_y<SIZE_Y; l_y++)
  {
    _Pragma("unroll")
    for(int l_z=0; l_z<SIZE_Z ; l_z++)
    { 
      reg_array[l_z][l_y] = reg_array[l_z+1][l_y];
    }
  }
}
template<class REAL, int SIZE_REG, int SIZE=SIZE_REG, int REG_BASE=0>
__device__ void __forceinline__ reg2global3d(
            REAL reg_array[SIZE_REG], REAL*dst,
            int global_z, int width_z,
            int global_y, int width_y,
            int global_x, int width_x,
            int tid_x)
{
  _Pragma("unroll")
  for(int l_y=0; l_y<SIZE; l_y++)
  {
    dst[global_z*width_x*width_y+(global_y+l_y)*width_x+global_x+tid_x]=reg_array[l_y+REG_BASE];
  }
}


\end{lstlisting}
\begin{lstlisting}[language=C,rulecolor=\color{black}, basicstyle=\tiny, caption=PERKS-based full 3D 7-pt stencil kernel including halo region management,captionpos=t]
#define HALO (1)
#define NOCACHE_Z (HALO)
template<class REAL, int halo, 
int LOCAL_ITEM_PER_THREAD, int LOCAL_TILE_X, const int reg_folder_z, bool UseSMCache, int BLOCKDIM=256>
__device__ __forceinline__ void kernel3d_general_inner(REAL * __restrict__ input, REAL * __restrict__ output, int width_z, int width_y, int width_x,REAL* l2_cache_i, REAL* l2_cache_o,  int iteration, int max_sm_flder) 
{
  #define LOCAL_TILE_Y (LOCAL_ITEM_PER_THREAD*BLOCKDIM/LOCAL_TILE_X)
  #define gdim_y (BLOCKDIM/LOCAL_TILE_X)  
  if(!UseSMCache) max_sm_flder=0;
  #define UseRegCache (reg_folder_z!=0)
  const int tile_x_with_halo=LOCAL_TILE_X+2*halo;
  const int tile_y_with_halo=LOCAL_TILE_Y+2*halo;
  stencilParaT;
  extern __shared__ char sm[];
  REAL* sm_rbuffer = (REAL*)sm+1;
  REAL* smbuffer_buffer_ptr[halo+1+isBOX];
  smbuffer_buffer_ptr[0]=sm_rbuffer;
  #pragma unroll
  for(int hl=1; hl<halo+1+isBOX; hl++)
  {
    smbuffer_buffer_ptr[hl]=smbuffer_buffer_ptr[hl-1]+tile_x_with_halo*tile_y_with_halo;
  }
  REAL* sm_space = sm_rbuffer+tile_x_with_halo*tile_y_with_halo*(halo+1+isBOX);
  REAL* boundary_buffer=sm_space+max_sm_flder*LOCAL_TILE_X*(LOCAL_TILE_Y);
  register REAL r_smbuffer[2*halo+1][REG_Y_SIZE_MOD];
  register REAL r_space[reg_folder_z<=0?1:reg_folder_z][LOCAL_ITEM_PER_THREAD];
  /***********************/
  const int tid_x = threadIdx.x%LOCAL_TILE_X;
  const int tid_y = threadIdx.x/LOCAL_TILE_X;
  const int dim_y = LOCAL_TILE_Y/LOCAL_ITEM_PER_THREAD;
  const int cpblocksize_y=(tile_y_with_halo)/dim_y;
  const int cpquotion_y=(tile_y_with_halo)%dim_y;
  const int index_y = LOCAL_ITEM_PER_THREAD*tid_y;
  const int cpbase_y = -halo+tid_y*cpblocksize_y+(tid_y<=cpquotion_y?tid_y:cpquotion_y);
  const int cpend_y = cpbase_y + cpblocksize_y + (tid_y<=cpquotion_y?1:0);
  const int ps_y = halo;
  const int ps_x = halo;
  const int p_x = blockIdx.x * LOCAL_TILE_X;
  const int p_y = blockIdx.y * LOCAL_TILE_Y;
  int blocksize_z=(width_z/gridDim.z);
  int z_quotient = width_z%gridDim.z;
  const int p_z =  blockIdx.z * (blocksize_z) + (blockIdx.z<=z_quotient?blockIdx.z:z_quotient);
  blocksize_z += (blockIdx.z<z_quotient?1:0);
  const int p_z_reg_start=p_z+NOCACHE_Z;
  const int p_z_sm_start=p_z+NOCACHE_Z + reg_folder_z;
  const int p_z_sm_end=p_z_sm_start+max_sm_flder;
  const int p_z_end = p_z + (blocksize_z);
  const int total_folder_z=max_sm_flder+reg_folder_z;
  const int boundary_east_step=0;
  const int boundary_west_step=(LOCAL_TILE_Y+isBOX*2)*(total_folder_z)*halo;
  const int boundary_north_step=boundary_west_step+(LOCAL_TILE_Y+isBOX*2)*(total_folder_z)*halo;
  const int boundary_south_step=boundary_north_step+TILE_X*total_folder_z*halo;
  const int l2_boundary_east_step=0;
  const int l2_boundary_west_step=width_y*halo*gridDim.x*total_folder_z*gridDim.z;
  const int l2_boundary_north_step=l2_boundary_west_step+width_y*halo*gridDim.x*total_folder_z*gridDim.z;
  const int l2_boundary_south_step=l2_boundary_north_step+width_x*halo*gridDim.y*total_folder_z*gridDim.z; 
  const int boundary_step_yz=(LOCAL_TILE_Y+isBOX*2)*total_folder_z;
  _Pragma("unroll")
  for(int cache_z=0; cache_z<reg_folder_z; cache_z++)
  {
    for(int l_y=0; l_y<LOCAL_ITEM_PER_THREAD; l_y++)
    {
      int local_y=l_y+LOCAL_ITEM_PER_THREAD*tid_y;
      r_space[cache_z][l_y]
        = input[(p_z_reg_start + cache_z)*width_x*width_y+(local_y+p_y)*width_x+p_x+tid_x];
    }
  }
  // global 2 sm cache
  for(int cache_z=0; cache_z<max_sm_flder; cache_z++)
  {
    for(int l_y=0; l_y<LOCAL_ITEM_PER_THREAD; l_y++)
    {
      int local_y=l_y+LOCAL_ITEM_PER_THREAD*tid_y;
      sm_space[cache_z*LOCAL_TILE_X*LOCAL_TILE_Y+local_y*LOCAL_TILE_X+tid_x]
        = input[(p_z_sm_start + cache_z)*width_x*width_y+(local_y+p_y)*width_x+p_x+tid_x];
    }
  }
  // boundary
  for(int cache_z=0; cache_z<max_sm_flder+reg_folder_z; cache_z++)
  {
    for(int l_y=threadIdx.x-isBOX; l_y<LOCAL_TILE_Y+isBOX; l_y+=blockDim.x)
    {
      int global_y=MIN(p_y+l_y,width_y-1);
      global_y=MAX(0,global_y);
      #pragma unroll
      for(int l_x=0; l_x<halo; l_x++)
      {
        //east
        int global_x = p_x+LOCAL_TILE_X+l_x;
        global_x = MIN(width_x-1,global_x);
        boundary_buffer[boundary_east_step + cache_z *  (LOCAL_TILE_Y+2*isBOX)*halo + (l_y+isBOX) + l_x * (LOCAL_TILE_Y+2*isBOX)] = input[(p_z+NOCACHE_Z+cache_z)*width_x*width_y+(global_y)*width_x+global_x];
        // //west
        global_x = p_x-halo+l_x;
        global_x = MAX(0,global_x);
        boundary_buffer[boundary_west_step + cache_z *  (LOCAL_TILE_Y+2*isBOX)*halo + (l_y+isBOX) + l_x *  (LOCAL_TILE_Y+2*isBOX)] = input[(p_z+NOCACHE_Z+cache_z)*width_x*width_y+(global_y)*width_x+global_x];
      }
    }
    for(int l_x=threadIdx.x; l_x<TILE_X; l_x+=blockDim.x)
    {
      int global_x = p_x+l_x;
      #pragma unroll
      for(int l_y=0; l_y<halo; l_y++)
      {
        //north
        int global_y = p_y + LOCAL_TILE_Y + l_y;
        global_y=MIN(global_y,width_y-1);
        boundary_buffer[boundary_north_step + cache_z * LOCAL_TILE_X * halo + (l_x) + l_y * LOCAL_TILE_X]= input[(p_z+NOCACHE_Z+cache_z)*width_x*width_y+(global_y)*width_x+global_x];
        //south
        global_y = p_y - halo + l_y;
        global_y=MAX(global_y,0);
        boundary_buffer[boundary_south_step + cache_z * LOCAL_TILE_X * halo + (l_x) + l_y * LOCAL_TILE_X]= input[(p_z+NOCACHE_Z+cache_z)*width_x*width_y+(global_y)*width_x+global_x];
      }
    }
  }
  // int smz_ind=0;
  cg::grid_group gg = cg::this_grid();
  for(int iter=0; iter<iteration; iter++)
  {
    // halo in(global, 0,halo)
    global2regs3d<REAL, 1+2*halo, LOCAL_ITEM_PER_THREAD>
      (input, r_smbuffer, p_z-halo,width_z, p_y+index_y, width_y, p_x, width_x,tid_x);
    global2sm<REAL, halo, -isBOX, halo + isBOX, halo+isBOX+1, 0, true, false> (input, smbuffer_buffer_ptr, p_x, p_y, p_z, width_x, width_y, width_z,tile_x_with_halo, ps_x,cpbase_y, cpend_y, 1,ps_y,LOCAL_TILE_X, tid_x);
    // // // reg->global
    if(UseRegCache)
    {
      _Pragma("unroll")
      for(int global_z=p_z, cache_z_reg=0; global_z<p_z_reg_start; global_z+=1, cache_z_reg++)
      {
        process_one_layer<REAL, halo, LOCAL_ITEM_PER_THREAD, BLOCKDIM, LOCAL_TILE_X, halo+1+isBOX, 2*halo+1,reg_folder_z==0?1:reg_folder_z, true,false, true, false>(input, output, smbuffer_buffer_ptr, r_smbuffer, global_z,  p_y,  p_x, width_z,  width_y,  width_x, ps_y, ps_x, tile_x_with_halo,cpbase_y, cpend_y, index_y,tid_x, tid_y, stencilParaInput,sm_space, 0, 0,r_space, cache_z_reg, 0,boundary_buffer, cache_z_reg, boundary_east_step, boundary_west_step, boundary_north_step, boundary_south_step,boundary_step_yz
        );
      }    
      // // reg->reg                    
      _Pragma("unroll")   
      for(int global_z=p_z_reg_start,cache_z_reg=halo; global_z<p_z_sm_start-halo; global_z+=1,cache_z_reg++)
      {
        process_one_layer<REAL, halo, LOCAL_ITEM_PER_THREAD, BLOCKDIM, LOCAL_TILE_X, halo+1+isBOX, 2*halo+1,reg_folder_z==0?1:reg_folder_z, true,true,true, true> (input, output, smbuffer_buffer_ptr,  r_smbuffer,global_z,  p_y,  p_x,width_z,  width_y,  width_x,ps_y, ps_x, tile_x_with_halo, cpbase_y, cpend_y, index_y,   tid_x, tid_y,stencilParaInput,sm_space, 0, 0,r_space, cache_z_reg,cache_z_reg-halo,boundary_buffer, cache_z_reg, boundary_east_step, boundary_west_step,boundary_north_step,boundary_south_step,boundary_step_yz );
      }
    }
    if((UseRegCache)&&UseSMCache)
    {
      _Pragma("unroll")
      for(int global_z=p_z_sm_start-halo, cache_z=0; global_z<p_z_sm_start; global_z+=1, cache_z++)
      {
        process_one_layer<REAL, halo, LOCAL_ITEM_PER_THREAD, BLOCKDIM, LOCAL_TILE_X, halo+1+isBOX, 2*halo+1,reg_folder_z==0?1:reg_folder_z, true,true,false, true>(input, output,  smbuffer_buffer_ptr, r_smbuffer, global_z,  p_y,  p_x,width_z,  width_y,  width_x,ps_y, ps_x, tile_x_with_halo,cpbase_y, cpend_y, index_y,tid_x, tid_y, stencilParaInput, sm_space, cache_z, 0, r_space, 0, cache_z+reg_folder_z-halo, boundary_buffer, cache_z+reg_folder_z,  boundary_east_step, boundary_west_step, boundary_north_step, boundary_south_step, boundary_step_yz );
      }
    }
    
    if((UseRegCache)&&!UseSMCache)
    {
       // // global -> (reg)
      _Pragma("unroll")
      for(int global_z=p_z_sm_start-halo, cache_z=0, cache_z_reg=reg_folder_z; global_z<p_z_sm_start; global_z+=1, cache_z++,cache_z_reg++)
      {
        process_one_layer<REAL, halo, LOCAL_ITEM_PER_THREAD, BLOCKDIM, LOCAL_TILE_X, halo+1+isBOX, 2*halo+1, reg_folder_z==0?1:reg_folder_z, false,true,false, true>(input, output,  smbuffer_buffer_ptr,  r_smbuffer,global_z,  p_y,  p_x, width_z,  width_y,  width_x,ps_y, ps_x, tile_x_with_halo, cpbase_y, cpend_y, index_y, tid_x, tid_y, stencilParaInput, sm_space, 0, 0,  r_space, 0, cache_z_reg-halo, boundary_buffer, cache_z+reg_folder_z,   boundary_east_step,boundary_west_step, boundary_north_step, boundary_south_step, boundary_step_yz
        );
      }
    }
    //register  boundary 
    //east and west 
    _Pragma("unroll")
    for(int l_z=0; l_z<reg_folder_z; l_z++)
    {
      if(tid_x>=LOCAL_TILE_X-halo)
      {
        int l_x=tid_x-LOCAL_TILE_X+halo;
        for(int l_y=0; l_y<LOCAL_ITEM_PER_THREAD;l_y+=1)
        {
          int local_y=l_y+LOCAL_ITEM_PER_THREAD*tid_y;
          //east
          boundary_buffer[boundary_east_step + (l_z) *  (LOCAL_TILE_Y+2*isBOX)*halo + (local_y+isBOX) + l_x * (LOCAL_TILE_Y+2*isBOX)]=r_space[l_z][l_y];
        }
      }
      if(tid_x<halo)
      {
        int l_x=tid_x;
        for(int l_y=0; l_y<LOCAL_ITEM_PER_THREAD;l_y+=1)
        {
          int local_y=l_y+LOCAL_ITEM_PER_THREAD*tid_y;
          //west
          boundary_buffer[boundary_west_step + (l_z) *  (LOCAL_TILE_Y+2*isBOX)*halo + (local_y+isBOX) + l_x * (LOCAL_TILE_Y+2*isBOX)]=r_space[l_z][l_y];
        }
      }
    }
    //north and south
    _Pragma("unroll")
    for(int l_z=0; l_z<reg_folder_z; l_z++)
    {
      
      int l_x=tid_x;
      #pragma unroll
      for(int l_y=0; l_y<halo; l_y++)
      {
        //south
        if(tid_y==0)
        {
          boundary_buffer[boundary_south_step + (l_z) *  (LOCAL_TILE_X)*halo + (l_x) + l_y * (LOCAL_TILE_X)] = r_space[l_z][l_y];
        }
        //north
        if(tid_y==dim_y-1)
        {
          boundary_buffer[boundary_north_step + (l_z) *  (LOCAL_TILE_X)*halo + (l_x) + (l_y) * (LOCAL_TILE_X)] = r_space[l_z][LOCAL_ITEM_PER_THREAD-halo+ l_y];
        } 
      }
    }
    //no need sync
    if(!UseRegCache&&UseSMCache)
    {
      // sm -> global
      _Pragma("unroll")
      for(int global_z=p_z_sm_start-halo, cache_z=0, cache_z_reg=reg_folder_z; global_z<p_z_sm_start; global_z+=1, cache_z++,cache_z_reg++)
      {
        process_one_layer<REAL, halo, LOCAL_ITEM_PER_THREAD, BLOCKDIM, LOCAL_TILE_X, halo+1+isBOX, 2*halo+1, reg_folder_z==0?1:reg_folder_z,true, false, false, false>(input, output,  smbuffer_buffer_ptr,  r_smbuffer, global_z,  p_y,  p_x,  width_z,  width_y,  width_x,ps_y, ps_x, tile_x_with_halo,cpbase_y, cpend_y, index_y, tid_x, tid_y, stencilParaInput, sm_space, cache_z, 0, r_space, 0, cache_z_reg-halo, boundary_buffer, cache_z+reg_folder_z, boundary_east_step, boundary_west_step, boundary_north_step, boundary_south_step, boundary_step_yz);
      }
    }

    if(UseSMCache)
    {
      // // // // sm->sm
      for(int global_z=p_z_sm_start, cache_z=halo; global_z<p_z_sm_end-halo; global_z+=1, cache_z++)
      {
        process_one_layer<REAL, halo, LOCAL_ITEM_PER_THREAD, BLOCKDIM, LOCAL_TILE_X, halo+1+isBOX, 2*halo+1, reg_folder_z==0?1:reg_folder_z, true,true> (input, output, smbuffer_buffer_ptr, r_smbuffer, global_z,  p_y,  p_x, width_z,  width_y,  width_x, ps_y, ps_x, tile_x_with_halo,cpbase_y, cpend_y, index_y,tid_x, tid_y, stencilParaInput, sm_space, cache_z, cache_z-halo, r_space, 0, 0, boundary_buffer, cache_z+reg_folder_z,  boundary_east_step, boundary_west_step, boundary_north_step, boundary_south_step, boundary_step_yz  );
      }
      // // // // // global->sm
      for(int global_z=p_z_sm_end-halo, cache_z=max_sm_flder; global_z<p_z_sm_end; global_z+=1, cache_z++)
      {
        process_one_layer<REAL, halo, LOCAL_ITEM_PER_THREAD, BLOCKDIM, LOCAL_TILE_X, halo+1+isBOX, 2*halo+1,reg_folder_z==0?1:reg_folder_z, false,true>(input, output, smbuffer_buffer_ptr,  r_smbuffer, global_z,  p_y,  p_x, width_z,  width_y,  width_x, ps_y, ps_x, tile_x_with_halo,  cpbase_y, cpend_y, index_y,  tid_x, tid_y, stencilParaInput, sm_space, 0, cache_z-halo );
      }

    }
    if(!UseSMCache&&!UseRegCache)
    {
      for(int global_z=p_z; global_z<p_z_sm_end; global_z+=1)
      {
        process_one_layer<REAL, halo, LOCAL_ITEM_PER_THREAD, BLOCKDIM,LOCAL_TILE_X, halo+1+isBOX, 2*halo+1>(input, output,  smbuffer_buffer_ptr,  r_smbuffer, global_z,  p_y,  p_x,  width_z,  width_y,  width_x, ps_y, ps_x, tile_x_with_halo,cpbase_y, cpend_y, index_y, tid_x, tid_y, stencilParaInput); 
      }
    }

    __syncthreads();
    //sm boundary
    //sm east and west
    _Pragma("unroll")
    for(int l_z=0; l_z<max_sm_flder; l_z++)
    {
      for(int l_x=tid_y; l_x<halo; l_x+=dim_y)
      {
        for(int l_y=tid_x; l_y<LOCAL_TILE_Y;l_y+=LOCAL_TILE_X)
        {
          //east
          boundary_buffer[boundary_east_step + (l_z+reg_folder_z) *  (LOCAL_TILE_Y+2*isBOX)*halo + (l_y+isBOX) + l_x * (LOCAL_TILE_Y+2*isBOX)] =sm_space[l_z*(LOCAL_TILE_Y)*LOCAL_TILE_X+(l_y)*LOCAL_TILE_X+LOCAL_TILE_X-halo+l_x];

          //west
          boundary_buffer[boundary_west_step + (l_z+reg_folder_z) *  (LOCAL_TILE_Y+2*isBOX)*halo + (l_y+isBOX) + l_x * (LOCAL_TILE_Y+2*isBOX)] = sm_space[l_z*(LOCAL_TILE_Y)*LOCAL_TILE_X+(l_y)*LOCAL_TILE_X+l_x];
        }
      }
    }
    //sm south and north
    _Pragma("unroll")
    for(int l_z=0; l_z<max_sm_flder; l_z++)
    {
      int l_x=tid_x;
      {
        for(int l_y=tid_y; l_y<halo; l_y+=dim_y)
        {
          //south
          {
            boundary_buffer[boundary_south_step + (l_z+reg_folder_z) *  (LOCAL_TILE_X)*halo + (l_x) + l_y * (LOCAL_TILE_X)]
              = sm_space[l_z*(LOCAL_TILE_Y)*LOCAL_TILE_X+(l_y)*LOCAL_TILE_X+l_x];
          }
          //north
          {
            boundary_buffer[boundary_north_step + (l_z+reg_folder_z) *  (LOCAL_TILE_X)*halo + (l_x) + (l_y) * (LOCAL_TILE_X)]
              = sm_space[l_z*(LOCAL_TILE_Y)*LOCAL_TILE_X+(l_y+LOCAL_TILE_Y-halo)*LOCAL_TILE_X+l_x];
          } 
        }
      }
    }
    // general version
    for(int global_z=p_z_sm_end; global_z<p_z_end; global_z+=1)
    {
      process_one_layer<REAL, halo, LOCAL_ITEM_PER_THREAD, BLOCKDIM, LOCAL_TILE_X, halo+1+isBOX, 2*halo+1> (input, output, smbuffer_buffer_ptr,  r_smbuffer, global_z,  p_y,  p_x, width_z,  width_y,  width_x, ps_y, ps_x, tile_x_with_halo, cpbase_y, cpend_y, index_y, tid_x, tid_y, stencilParaInput); 
    }
    __syncthreads();
    if(iter>=iteration-1)break;
    //deal with east and west boundary
    //store to global memory in l2 cache pointer (hopefully)  
   
    {
      int bid_x=blockIdx.x;
      int gdimx=gridDim.x;
      int bid_y=blockIdx.y;
      int gdimy=gridDim.y;
      int bid_z=blockIdx.z;
      //x
      if(gdim_y>=2)
      {
        if(tid_y<dim_y/2)
        {
          for(int l_x=tid_y; l_x<halo; l_x+=dim_y/2)
          {
            //z
            for(int l_z=0; l_z<total_folder_z; l_z++)
            {
              //y
              for(int l_y=tid_x; l_y<LOCAL_TILE_Y; l_y+=LOCAL_TILE_X)
              {
                // //west
                l2_cache_o[l2_boundary_west_step + l_y + bid_y*LOCAL_TILE_Y + (l_x + bid_x*halo)*width_y + (l_z+bid_z*total_folder_z)*width_y*gdimx*halo ] 
                = boundary_buffer[boundary_west_step + (l_z) *  (LOCAL_TILE_Y+2*isBOX)*halo + (l_y+isBOX) + l_x * (LOCAL_TILE_Y+2*isBOX)];
              }
            }
          }
        }
        else
        {
          for(int l_x=tid_y-dim_y/2; l_x<halo; l_x+=dim_y/2)
          {
            //z
            for(int l_z=0; l_z<total_folder_z; l_z++)
            {
              //y
              for(int l_y=tid_x; l_y<LOCAL_TILE_Y; l_y+=LOCAL_TILE_X)
              {
                //east
                l2_cache_o[l2_boundary_east_step + l_y + bid_y*LOCAL_TILE_Y + (l_x + bid_x*halo)*width_y + (l_z+bid_z*total_folder_z)*width_y*gdimx*halo ]  
                = boundary_buffer[boundary_east_step + (l_z) *  (LOCAL_TILE_Y+2*isBOX)*halo + (l_y+isBOX) + l_x * (LOCAL_TILE_Y+2*isBOX)];
              }
            }
          }
        }
      }
      else
      {
        {
          for(int l_x=tid_y; l_x<halo; l_x+=1)
          {
            //z
            for(int l_z=0; l_z<total_folder_z; l_z++)
            {
              //y
              for(int l_y=tid_x; l_y<LOCAL_TILE_Y; l_y+=LOCAL_TILE_X)
              {
                // //west
                l2_cache_o[l2_boundary_west_step + l_y + bid_y*LOCAL_TILE_Y + (l_x + bid_x*halo)*width_y + (l_z+bid_z*total_folder_z)*width_y*gdimx*halo ] 
                = boundary_buffer[boundary_west_step + (l_z) *  (LOCAL_TILE_Y+2*isBOX)*halo + (l_y+isBOX) + l_x * (LOCAL_TILE_Y+2*isBOX)];
              }
            }
          }
        }
        {
          for(int l_x=tid_y; l_x<halo; l_x+=1)
          {
            //z
            for(int l_z=0; l_z<total_folder_z; l_z++)
            {
              //y
              for(int l_y=tid_x; l_y<LOCAL_TILE_Y; l_y+=LOCAL_TILE_X)
              {
                //east
                l2_cache_o[l2_boundary_east_step + l_y + bid_y*LOCAL_TILE_Y + (l_x + bid_x*halo)*width_y + (l_z+bid_z*total_folder_z)*width_y*gdimx*halo ]  
                = boundary_buffer[boundary_east_step + (l_z) *  (LOCAL_TILE_Y+2*isBOX)*halo + (l_y+isBOX) + l_x * (LOCAL_TILE_Y+2*isBOX)];
              }
            }
          }
        }
      }
      // // //north south
      if(gdim_y>=2)
      {
        if(tid_y<dim_y/2)
        {
          for(int l_y=tid_y; l_y<halo; l_y+=dim_y/2)
          {
            //z
            for(int l_z=0; l_z<total_folder_z; l_z++)
            {
              //y
              {
                int l_x=tid_x;
                // //north
                l2_cache_o[l2_boundary_north_step + l_x + bid_x * TILE_X + (l_y + bid_y * halo) * width_x + (l_z + bid_z * total_folder_z) * width_x * gdimy*halo ] 
                  = boundary_buffer[boundary_north_step + (l_z) *  (LOCAL_TILE_X)*halo + (l_x) + l_y * (LOCAL_TILE_X)];
              }
            }
          }
        }
        else
        {
          for(int l_y=tid_y-dim_y/2; l_y<halo; l_y+=dim_y/2)
          {
            //z
            for(int l_z=0; l_z<total_folder_z; l_z++)
            {
              //y
              {
                int l_x=tid_x;
                // south 
                l2_cache_o[l2_boundary_south_step + l_x + bid_x * TILE_X + (l_y + bid_y * halo) * width_x + (l_z + bid_z * total_folder_z) * width_x * gdimy*halo ]  
                  = boundary_buffer[boundary_south_step + (l_z) *  (LOCAL_TILE_X)*halo + (l_x) + l_y * (LOCAL_TILE_X)];
              }
            }
          }
        }
      }
      else
      {
        // if(tid_y<dim_y/2)
        {
          for(int l_y=tid_y; l_y<halo; l_y+=1)
          {
            //z
            for(int l_z=0; l_z<total_folder_z; l_z++)
            {
              //y
              {
                int l_x=tid_x;
                // //north
                l2_cache_o[l2_boundary_north_step + l_x + bid_x * TILE_X + (l_y + bid_y * halo) * width_x + (l_z + bid_z * total_folder_z) * width_x * gdimy*halo ] 
                  = boundary_buffer[boundary_north_step + (l_z) *  (LOCAL_TILE_X)*halo + (l_x) + l_y * (LOCAL_TILE_X)];
              }
            }
          }
        }
        // else
        {
          for(int l_y=tid_y; l_y<halo; l_y+=1)
          {
            //z
            for(int l_z=0; l_z<total_folder_z; l_z++)
            {
              //y
              {
                int l_x=tid_x;
                // south 
                l2_cache_o[l2_boundary_south_step + l_x + bid_x * TILE_X + (l_y + bid_y * halo) * width_x + (l_z + bid_z * total_folder_z) * width_x * gdimy*halo ]  
                  = boundary_buffer[boundary_south_step + (l_z) *  (LOCAL_TILE_X)*halo + (l_x) + l_y * (LOCAL_TILE_X)];
              }
            }
          }
        }
      }

    }

    gg.sync();
    //load frm global memory in l2 cache pointer (hopefully)
    REAL* tmp_ptr =output;
    output=input;
    input=tmp_ptr;

    tmp_ptr=l2_cache_o;
    l2_cache_o=l2_cache_i;
    l2_cache_i=tmp_ptr;

    {

      // int bid_y=blockIdx.x/gdim_x;
      int bid_x=blockIdx.x;
      int gdimx=gridDim.x;

      int bid_y=blockIdx.y;
      int gdimy=gridDim.y;
      
      int bid_z=blockIdx.z;
      //x
      if(gdim_y>=2)
      {
        if(tid_y<dim_y/2)
        {
          for(int l_x=tid_y; l_x<halo; l_x+=dim_y/2)
          {
            //z
            for(int l_z=0; l_z<total_folder_z; l_z++)
            {
              //y
              for(int l_y=tid_x-isBOX; l_y<LOCAL_TILE_Y+isBOX; l_y+=LOCAL_TILE_X)
              {
                int l2_cache_l_y=MAX(l_y+ bid_y*LOCAL_TILE_Y,0);
                l2_cache_l_y=MIN(l2_cache_l_y,width_y-1);

                //east
                boundary_buffer[boundary_east_step + (l_z) *  (LOCAL_TILE_Y+2*isBOX)*halo+ (l_y+isBOX) + l_x * (LOCAL_TILE_Y+2*isBOX)] =
                  (bid_x==gdimx-1?
                  l2_cache_i[l2_boundary_east_step+ l2_cache_l_y  + ((halo-1) + bid_x*halo)*width_y + (l_z+bid_z*total_folder_z)*width_y*gdimx*halo ]  
                 :
                 l2_cache_i[l2_boundary_west_step+l2_cache_l_y  + (l_x + (bid_x+1)*halo)*width_y + (l_z+bid_z*total_folder_z)*width_y*gdimx*halo  ]
                 )
                 ;

              }
            }
          }
        }
        else
        {
          for(int l_x=tid_y-dim_y/2; l_x<halo; l_x+=dim_y/2)
          {
            //z
            for(int l_z=0; l_z<total_folder_z; l_z++)
            {
              //y
              for(int l_y=tid_x-isBOX; l_y<LOCAL_TILE_Y+isBOX; l_y+=LOCAL_TILE_X)
              {
                int l2_cache_l_y=MAX(l_y+ bid_y*LOCAL_TILE_Y,0);
                l2_cache_l_y=MIN(l2_cache_l_y,width_y-1);

                //west
                boundary_buffer[boundary_west_step + (l_z) *  (LOCAL_TILE_Y+2*isBOX)*halo + (l_y+isBOX) + l_x * (LOCAL_TILE_Y+2*isBOX)] =
                  (bid_x==0?
                    l2_cache_i[l2_boundary_west_step+ l2_cache_l_y  + (0 + bid_x*halo)*width_y + (l_z+bid_z*total_folder_z)*width_y*gdimx*halo ] 
                    :
                    l2_cache_i[l2_boundary_east_step+ l2_cache_l_y  + (l_x + (bid_x-1)*halo)*width_y + (l_z+bid_z*total_folder_z)*width_y*gdimx*halo ])
                    ;
              }
            }
          }
        }
        if(tid_y<dim_y/2)
        {
          for(int l_y=tid_y; l_y<halo; l_y+=dim_y/2)
          {
            //z
            for(int l_z=0; l_z<total_folder_z; l_z++)
            {
              //y
              {
                int l_x=tid_x;
                if(tid_y<halo)
                //north
                boundary_buffer[boundary_north_step + (l_z) *  (LOCAL_TILE_X)*halo + (l_x) + l_y * (LOCAL_TILE_X)] =
                  (bid_y==gdimy-1?
                 boundary_buffer[boundary_north_step + (l_z) *  (LOCAL_TILE_X)*halo + (l_x) + (halo-1) * (LOCAL_TILE_X)]
                 :
                 l2_cache_i[l2_boundary_south_step + l_x + bid_x * LOCAL_TILE_X + (l_y + (bid_y+1) * halo) * width_x + (l_z + bid_z * total_folder_z) * width_x * gdimy*halo  ]
                 )
                 ;
                //south
                boundary_buffer[boundary_south_step + (l_z) *  (LOCAL_TILE_X)*halo + (l_x) + l_y * (LOCAL_TILE_X)] =
                  (bid_y==0?
                    boundary_buffer[boundary_south_step + (l_z) *  (LOCAL_TILE_X)*halo + (l_x) + 0 * (LOCAL_TILE_X)]
                    :
                    l2_cache_i[l2_boundary_north_step + l_x + bid_x * LOCAL_TILE_X + (l_y + (bid_y-1) * halo) * width_x + (l_z + bid_z * total_folder_z) * width_x * gdimy*halo ])
                    ;
              }
            }
          }
        }
        else
        {
          for(int l_y=tid_y-dim_y/2; l_y<halo; l_y+=dim_y/2)
          {
            //z
            for(int l_z=0; l_z<total_folder_z; l_z++)
            {
              //y
              {
                int l_x=tid_x;
                //north
                boundary_buffer[boundary_north_step + (l_z) *  (LOCAL_TILE_X)*halo + (l_x) + l_y * (LOCAL_TILE_X)] =
                  (bid_y==gdimy-1?
                 boundary_buffer[boundary_north_step + (l_z) *  (LOCAL_TILE_X)*halo + (l_x) + (halo-1) * (LOCAL_TILE_X)]
                 :
                 l2_cache_i[l2_boundary_south_step + l_x + bid_x * LOCAL_TILE_X + (l_y + (bid_y+1) * halo) * width_x + (l_z + bid_z * total_folder_z) * width_x * gdimy*halo  ]
                 )
                 ;

              }
            }
          }
        }

      }
      else
      {
        // if(tid_y<dim_y/2)
        {
          for(int l_x=tid_y; l_x<halo; l_x+=1)
          {
            //z
            for(int l_z=0; l_z<total_folder_z; l_z++)
            {
              //y
              for(int l_y=tid_x-isBOX; l_y<LOCAL_TILE_Y+isBOX; l_y+=LOCAL_TILE_X)
              {
                int l2_cache_l_y=MAX(l_y+ bid_y*LOCAL_TILE_Y,0);
                l2_cache_l_y=MIN(l2_cache_l_y,width_y-1);

                //east
                boundary_buffer[boundary_east_step + (l_z) *  (LOCAL_TILE_Y+2*isBOX)*halo+ (l_y+isBOX) + l_x * (LOCAL_TILE_Y+2*isBOX)] =
                  (bid_x==gdimx-1?
                  l2_cache_i[l2_boundary_east_step+ l2_cache_l_y  + ((halo-1) + bid_x*halo)*width_y + (l_z+bid_z*total_folder_z)*width_y*gdimx*halo ]  
                 :
                 l2_cache_i[l2_boundary_west_step+l2_cache_l_y  + (l_x + (bid_x+1)*halo)*width_y + (l_z+bid_z*total_folder_z)*width_y*gdimx*halo  ]
                 )
                 ;

              }
            }
          }
        }
        // else
        {
          for(int l_x=tid_y; l_x<halo; l_x+=1)
          {
            //z
            for(int l_z=0; l_z<total_folder_z; l_z++)
            {
              //y
              for(int l_y=tid_x-isBOX; l_y<LOCAL_TILE_Y+isBOX; l_y+=LOCAL_TILE_X)
              {
                int l2_cache_l_y=MAX(l_y+ bid_y*LOCAL_TILE_Y,0);
                l2_cache_l_y=MIN(l2_cache_l_y,width_y-1);

                //west
                boundary_buffer[boundary_west_step + (l_z) *  (LOCAL_TILE_Y+2*isBOX)*halo + (l_y+isBOX) + l_x * (LOCAL_TILE_Y+2*isBOX)] =
                  (bid_x==0?
                    l2_cache_i[l2_boundary_west_step+ l2_cache_l_y  + (0 + bid_x*halo)*width_y + (l_z+bid_z*total_folder_z)*width_y*gdimx*halo ] 
                    :
                    l2_cache_i[l2_boundary_east_step+ l2_cache_l_y  + (l_x + (bid_x-1)*halo)*width_y + (l_z+bid_z*total_folder_z)*width_y*gdimx*halo ])
                    ;
              }
            }
          }
        }
        {
          for(int l_y=tid_y; l_y<halo; l_y+=1)
          {
            //z
            for(int l_z=0; l_z<total_folder_z; l_z++)
            {
              //y
              {
                int l_x=tid_x;
                if(tid_y<halo)
                //north
                boundary_buffer[boundary_north_step + (l_z) *  (LOCAL_TILE_X)*halo + (l_x) + l_y * (LOCAL_TILE_X)] =
                  (bid_y==gdimy-1?
                 boundary_buffer[boundary_north_step + (l_z) *  (LOCAL_TILE_X)*halo + (l_x) + (halo-1) * (LOCAL_TILE_X)]
                 :
                 l2_cache_i[l2_boundary_south_step + l_x + bid_x * LOCAL_TILE_X + (l_y + (bid_y+1) * halo) * width_x + (l_z + bid_z * total_folder_z) * width_x * gdimy*halo  ]
                 )
                 ;
                //south
                boundary_buffer[boundary_south_step + (l_z) *  (LOCAL_TILE_X)*halo + (l_x) + l_y * (LOCAL_TILE_X)] =
                  (bid_y==0?
                    boundary_buffer[boundary_south_step + (l_z) *  (LOCAL_TILE_X)*halo + (l_x) + 0 * (LOCAL_TILE_X)]
                    :
                    l2_cache_i[l2_boundary_north_step + l_x + bid_x * LOCAL_TILE_X + (l_y + (bid_y-1) * halo) * width_x + (l_z + bid_z * total_folder_z) * width_x * gdimy*halo ])
                    ;
              }
            }
          }
        }
        {
          for(int l_y=tid_y; l_y<halo; l_y+=1)
          {
            //z
            for(int l_z=0; l_z<total_folder_z; l_z++)
            {
              //y
              {
                int l_x=tid_x;

                //north
                boundary_buffer[boundary_north_step + (l_z) *  (LOCAL_TILE_X)*halo + (l_x) + l_y * (LOCAL_TILE_X)] =
                  (bid_y==gdimy-1?
                 boundary_buffer[boundary_north_step + (l_z) *  (LOCAL_TILE_X)*halo + (l_x) + (halo-1) * (LOCAL_TILE_X)]
                 :
                 l2_cache_i[l2_boundary_south_step + l_x + bid_x * LOCAL_TILE_X + (l_y + (bid_y+1) * halo) * width_x + (l_z + bid_z * total_folder_z) * width_x * gdimy*halo  ]
                 )
                 ;

              }
            }
          }
        }
      }
      __syncthreads();
    }
  }

  for(int global_z=p_z_reg_start, cache_z_reg=halo; global_z<p_z_sm_start; global_z+=1, cache_z_reg++)
  {
      _Pragma("unroll")
      for(int l_y=0; l_y<LOCAL_ITEM_PER_THREAD; l_y++)
      {
        int local_y=l_y+LOCAL_ITEM_PER_THREAD*tid_y;

        output[global_z*width_x*width_y+(p_y+local_y)*width_x+p_x+tid_x]  = r_space[cache_z_reg-halo][l_y];
      }  
  } 
  for(int global_z=p_z_sm_start, cache_z=halo; global_z<p_z_sm_end; global_z+=1, cache_z++)
  {
      _Pragma("unroll")
      for(int l_y=0; l_y<LOCAL_ITEM_PER_THREAD; l_y++)
      {
        int local_y=l_y+LOCAL_ITEM_PER_THREAD*tid_y;

        output[global_z*width_x*width_y+(p_y+local_y)*width_x+p_x+tid_x]  =
          sm_space[(cache_z-halo)*LOCAL_TILE_X*LOCAL_TILE_Y+(local_y)*LOCAL_TILE_X+tid_x];
      }  
  }
 
  #undef UseRegCache
  #undef LOCAL_TILE_Y
  #undef gdim_y
}
\end{lstlisting}

% \appendix
